# Supplementary material for: On Separation Logic, Computational Independence, and Pseudorandomness (Extended Version)
Source: arXiv:2405.11987 source file (2024-05-20)
Supplement: Supplementary file 1 [file appendix.tex]

\subsection{tmp}

\DD{The following remark is a consequence of Remark 4, Remark 6 is just used once, so it can be inlined.}
% \begin{rem}
%   \label{rem:suppbackproj}
%   For every $\nat\in \NN$, and every $\memone\in \supp((\rsone_{\renvone \to \renvtwo})_\nat)$,
%   there is $\overline \memone \in \supp (\rsone_\nat)$ such that
%   $\overline \memone\restr{\dom(\renvtwo)}=\memone$.
% \end{rem}
% \begin{proof}
%   Assume that the conclusion does not hold, i.e. there is not
%   $\overline \memone \in \supp (\rsone_\nat)$
%   such that $\overline \memone\restr{\dom(\renvtwo)}=\memone$.
%   But observe that
%   \[
%     \bind {\rsone_\nat}{\memtwo \mapsto \unit{\memtwo\restr{\dom(\renvtwo)}}}(\memone)
%   =  \sum_{\memtwo \in \supp(\rsone_\nat)}\rsone_\nat(\memtwo) \cdot \unit{\memtwo\restr{\dom(\renvtwo)}}(\memone)
%   \]
%   In particular, for every term of the sum,
%   the second factor is equal to zero, so the whole
%   sum is equal to zero. This contradicts the premise.
% \end{proof}

\subsubsection{Properties of $\ind$ and $\ext$}
\label{sec:appindext}

\subsubsection{Properties of \CBI}
\label{sec:appcbi}

\subsection{Proofs from section \ref{sec:inference}}
\label{sec:appinference}

In this section, we prove the soundness of the Hoare Logic
introduced in section \ref{sec:inference} and we employ
this logic to show the correctness of the POTP encryption scheme

\subsubsection{Proofs from subsection \ref{subsec:rules}}
\label{sec:apprules}

\subsection{Pseudo-random Key Stretching}
\label{sec:appstretch}

In this section we start by showing the soundness of the axioms
\eqref{eq:axsplit} and \eqref{eq:axmerge}, later, we show how
the triple
\[
  \hot {\tyf{\ud k}{k:\stng \nat} \sep \Sep_{i=0}^h \top^{\renvthree_i}} {\binjudg {\renvone_h} {\EXP[h]}}{\ud {s_{h+1}}}.
\]
can be assessed.

For completeness's sake, we start by defining the
environment $\renvone$.
\begin{gather*}
  \begin{aligned}
    \renvone_h(k)&= \nat &\forall 0\le i \le h. \renvone_h(\rvarone_i)&=\nat+1\\
    \forall 0\le i \le h. \renvone_h (b_i) &= \bool &  \renvone_h({s_{i}})(k)&= \nat +i.
  \end{aligned}\\
  \renvone_h(\rvartwo_{h+1}) = \nat+h+1
\end{gather*}

We start by defining some families of environments that will be employed in
the following. Together with the family $\{\renvone_h\}_{h\in \NN}$, that has already
been defined, we introduce the family $\{\overline \renvone_h\}_{h\in \NN}$,
which is pointwise identical to the former one, but is undefined on $\rvartwo_i$
for $0\le i\le h+1$. For every $i \in \NN$, we define
$\renvtwo_i$ as the environment which is equal to $\renvone_h$,
but all the $\rvarone_j$ and $b_j$ for $0\le j <i$ are undefined.
Finally, the family $\{\renvfour_h\}_{h \in \NN}$ is defined as follows:
\begin{align*}
  \renvfour_0 &\defsym \rvartwo_1: \stng{\nat+1}, k: \stng{\nat}, b_0: \bool,\\ 
  \renvfour_{i} &\defsym \rvartwo_{i+1}: \stng{\nat+i+1}, \rvartwo_{i}: \stng{\nat+i}, b_i: \bool, & i \neq 0
\end{align*}

With the definition above, we can start showing
the construction of the trees $\juone_i$ such that:
% \[
%   \juone_i \deriv \hot {\ud k\sep \tyf \top {\renvtwo_i}} {\binjudg {\renvone_h} {\prgone_i}}{\tyf{\ud k}{k:\stng \nat} \sep \ud {b_i}^{b_i:\bool}}.
% \]
%
% In order to do so, we employ the trees $\juone_i^1$, $\juone_i^2$
% and $\juone_i^3$ in \Cref{fig:juonei}. Their construction requires the
% following auxiliary result.
% %
% \begin{rem}
%   \label{rem:juonei1}
%   For every $\sttwo \in \sem {\renvtwo_i}{}$, if:
%   \[
%     \sr \sttwo {\tyf{\espl s {g(k)}}{\renvtwo_i} \land \tyf{\ud k}{k:\stng \nat}},
%   \]
%   then:
%   \[
%     \sr \sttwo{\tyf{\ud s}{\renvtwo_i}}
%   \]
% \end{rem}
% \begin{proof}
%   With \Cref{lemma:prekm}, we show:
%   \[
%     \sr \sttwo {\tyf{\espl s {g(k)}}{\renvtwo_i} \land \tyf{\ud k}{\renvtwo_i}}.
%   \]
%   Then the claim is shown with axioms (W1), (W2), (U1) and \eqref{eq:axpotp}.
% \end{proof}

% These trees can be put together with two applications of the $\RSEQ$ rule.
% This produces the triple 
% \[
%   \hot {\ud k} {\binjudg {\renvtwo_i} {\prgone_i}}
%   {\fone}.
% \]
% where $\fone$ is a shorthand for:
% %
% \[
%   {\tyf{\espl {k} {\tail({\rvarone_i})}}{\renvtwo_i} \land\tyf{\espl {b_i} {\head({\rvarone_i})}}{\renvtwo_i} \land \tyf{\ud {\rvarone_i}}{\renvtwo_i}},
% \]
% %
% On this triple, we can apply the $\RWEAK$ rule
% and \eqref{eq:axsplit} in order to obtain the conclusion
% \[
%   \tyf{\tyf{\ud{b_i} }{b_i:\bool} \sep \tyf{\ud k}{k:\stng\nat}}{\renvtwo_i},
% \]

% With an application of the $\RFRAME$ rule, we conclude the validity of the triple
\[
  \hotj{\tyf{\fone_i^h}{\renvone_h}}{\binjudg {\renvone_h} {\prgone_i} }{\tyf{\fone_{i+1}^h}{\renvone_h}}
\]
where
\begin{align*} 
  \fone_i^h &=\tyf{\ud k}{k:\stng \nat}\sep\;\;\smashoperator[lr]{\Sep_{j=0}^{i-1}}\;\; \tyf{\ud{b_j}}{b_j:\bool}\sep \;\; \top^{\renvtwo_i}%\\
 % \ftwo_i^h &=\tyf{\tyf{\ud{b_i} }{{b_i}:\bool} \sep \tyf{\ud k}{k:\stng\nat}}{\renvtwo_i}\sep\\&\quad \quad \quad \quad \quad \left( \smashoperator[r]{\Sep_{j=i+1}^h}\;\; \top^{\renvthree_j}\sep\;\;\smashoperator[lr]{\Sep_{j=0}^{i-1}}\;\; \tyf{\ud{b_i}}{b_i:\bool}\right).
\end{align*}
% With an application of the weakening rule, we conclude that the triple
% \[
%   \hotj{\tyf{\fone_i^h}{\renvone_h}}{\binjudg {\renvone_h} {\prgone_i} }{\tyf{\fone_{i+1}^h}{\renvone_h}}
% \]
% is valid. This comes from the observation that:
% \[
%   \srenv {{\renvtwo_i}}\stone {{\tyf{\ud{b_i} }{{b_i}:\bool}
%       \sep \tyf{\ud k}{k:\stng \nat}}
%   }
% \]
% has as consequence:
% \[
%   \srenv {(\renvtwo_i)_{b_i, k}} {\stone_{\renvtwo_i\to (\renvtwo_i)_{b_i, k}}} {\tyf{{\tyf{\ud{b_i} }{{b_i}:\bool}
%       \sep \tyf{\ud k}{k:\stng \nat}}
%   }{(\renvtwo_i)_{b_i, k}}}
% \]
% and that 
% \[
%   \srenv {{\renvtwo_{i+1}}}\stone {{\tyf{\ud{k} }{k:\stng \nat}
%       \sep \tyf{\top}{(\renvthree_{i+1})}}
%   }
% \]
% has as consequence
% \(
%   \srenv {{\renvtwo_{i+1}}}\stone {{{\ud{k} }}
%   }.
% \)
% Both the results follow from \Cref{cor:restriction}. Then, the other steps of the proof are basically rearrangements of the terms in $\ftwo_i$ justified by  \Cref{rem:conjasscomm}, which shows the associative and commutative property of $\sep$.
% %
With multiple applications of the $\RSEQ$ rule, we can show the triple
\[
  \hotj{\tyf{\fone_0^h}{\renvone_h}}{\binjudg {\renvone_h} {\prgone_h} }{\tyf{\fone_{h+1}^h}{\renvone_h}}.
  \tag{$*$}
\]
\noindent
Observe that $\fone_{h+1}^h$ corresponds to:
\[
\tyf{\ud k}{k:\stng \nat}\sep\;\;\smashoperator[lr]{\Sep_{j=0}^{h}}\;\; \tyf{\ud{b_j}}{b_j:\bool}\sep \;\; \top^{\renvtwo_{h+1}}
\]

Because of \Cref{rem:conjasscomm}, we observe that $\fone_{h+1}^h$ is the following one:
\[
\left(\tyf{\ud k}{k:\stng \nat}\sep \;\; \top^{\renvtwo_{h+1}}\right)\sep\left({\Sep_{j=0}^{h}}\;\; \tyf{\ud{b_j}}{b_j:\bool}\right)
\]
This consists in an application of the $\RWEAK$ rule. With application of the rule $\SDASS$, we can obtain the triple
\begin{gather*}
  \vdash \vhot{\left(\tyf{\ud k}{k:\stng \nat}\sep \;\; \top^{\renvtwo_{h+1}}\right)\sep\left({\Sep_{j=0}^{h}}\;\; \tyf{\ud{b_j}}{b_j:\bool}\right)
  }
  {\binjudg{\renvtwo_{h+1}, k:\stng\nat} {\ass {\rvartwo_0} k}}
  {\big(\tyf{\ud k \land \espl {\rvartwo_0} k}{k, \rvartwo_0:\stng \nat}\sep\\ \;\; \top^{\renvtwo_{h+1}\setminus\{\rvartwo_0:\stng\nat\}}\big)\sep\left({\Sep_{j=0}^{h}}\;\; \tyf{\ud{b_j}}{b_j:\bool}\right)
  }
\end{gather*}

By means of the $\RWEAK$ rule and axioms (W1), (W2) and (U1), we can rewrite the conclusion as follows:
$\left(\tyf{\ud  {\rvartwo_0} }{k, \rvartwo_0:\stng \nat}\sep \;\; \top^{\renvtwo_{h+1}\setminus\{\rvartwo_0:\stng\nat\}}\right)\sep\left({\Sep_{j=0}^{h}}\;\; \tyf{\ud{b_j}}{b_j:\bool}\right)$

%\DD{give a name to renvtwo\_h+1 - s\_i}

With another application of the $\RWEAK$ rule, we can produce the following triple:

\begin{gather*}
  \vdash \vhot{\left(\tyf{\ud k}{k:\stng \nat}\sep \;\; \top^{\renvtwo_{h+1}}\right)\sep\left({\Sep_{j=0}^{h}}\;\; \tyf{\ud{b_j}}{b_j:\bool}\right)
  }
  {\binjudg{\renvtwo_{h+1}, k:\stng\nat} {\ass {\rvartwo_0} k}}
  {\left(\tyf{\ud {\rvartwo_0}}{k, \rvartwo_0:\stng \nat}\right)\sep\left({\Sep_{j=0}^{h}}\;\; \tyf{\ud{b_j}}{b_j:\bool}\right)
  }
\end{gather*}

Finally, with \Cref{lemma:prekm} and \Cref{lemma:extcompcomp} we can simplify the conclusion one further step, to obtain:

\begin{gather*}
  \vdash \vhot{\left(\tyf{\ud k}{k:\stng \nat}\sep \;\; \top^{\renvtwo_{h+1}}\right)\sep\left({\Sep_{j=0}^{h}}\;\; \tyf{\ud{b_j}}{b_j:\bool}\right)
  }
  {\binjudg{\renvtwo_{h+1}, k:\stng\nat} {\ass {\rvartwo_0} k}
}  {\left(\tyf{\ud {\rvartwo_0}}{\rvartwo_0:\stng \nat}\right)\sep\left({\Sep_{j=0}^{h}}\;\; \tyf{\ud{b_j}}{b_j:\bool}\right)
  }
\end{gather*}

Observe that this can be put in a chain of applications of the $\RSEQ$
rule to show:

\begin{gather*}
  \vdash \vhot {\ud k  \sep \tyf \top{\renvtwo_0}} {\binjudg{\renvone_h}\prgone_0;\ldots;\prgone_h;\ass{\rvartwo_0} k}
  {\left(\tyf{\ud {\rvartwo_0}}{\rvartwo_0:\stng \nat}\right)\sep\left({\Sep_{j=0}^{h}}\;\; \tyf{\ud{b_j}}{b_j:\bool}\right)
  }
\end{gather*}
We continue by deifning the formula $\ftwo_i^h$ as follows:

\[
  \ftwo_i^h\defsym \left(\tyf{\ud {\rvartwo_i}}{\rvartwo_i:\stng {\nat+i}}\right)\sep\left({\Sep_{j=i}^{h}}\;\; \tyf{\ud{b_j}}{b_j:\bool}\right)
\]

Then, for every $\prgtwo_i$, for $0\le i\le h$, we build the
$\jutwo_i$ such that

\[
  \jutwo_i \deriv  \hotj {\ftwo_i^h} {\binjudg {\renvone_h} {\prgtwo_i}} {\ftwo_{i+1}^h}  
\]

These trees are descried in \Cref{fig:jutwoi} and can be combined by means of multiple applications of the $\RSEQ$ rule, this produces as conclusion the formula ${\ftwo_{h+1}^h}$, i.e. ${\ud {\rvartwo_{h+1}}{}}$. 

All these trees can
be combined with the $\RSEQ$ rule to prove the triple
\[
  \hot{\top}{\binjudg {\renvone_h} {\ass {s_1} {\concat_{\nat, 1}(k,{b_0})}\semic
      \seq{\seq{\prgtwo_{1}}\ldots}{\prgtwo_{h}}
    }
  }
  {
    \tyf{\ud{\rvartwo_{h+1}}}{\renvone_h}
  }
\]
\noindent
This triple is obtained with multiple applications of the $\RSEQ$ rule
to the family of trees $\jutwo_0, \ldots, \jutwo_h$.
%
% The most important
% step of these proofs is the application of the $\RWEAK$ rule
% with \Cref{lemma:expmergetech1} (for $\jutwo_0$)
% or \Cref{lemma:expmergetech2} (for the other trees).
% In turn, these lemmas use \eqref{eq:axmerge} to show that
% the string $\rvartwo_{i+1}$ is computationally uniform.
% and \Cref{lemma:sepdombigger} to show the independence of that
% string with all the $b_j$ for $i < j \le h$.
%
The claim is shown with of an application of the
$\RSEQ$ rule to the last triple and $(*)$.

\subsection{Proofs from \Cref{sec:compindep}}
\label{sec:proofencryption}
